# Supplementary material for: Low-entropy states of neutral atoms in polarization-synthesized optical lattices
Source: arXiv:1608.02410 ancillary file (2016-11-28)
Supplement: Supplementary file 1 [file SupplementalMaterial.pdf]

# Supplemental Material for: Low-entropy states of neutral atoms in polarization-synthesized optical lattices

Carsten Robens[1,†], Jonathan Zopes[1,†], Wolfgang Alt[1], Stefan Brakhane[1], Dieter Meschede[1], and Andrea Alberti[1,*]
[1]*Institut für Angewandte Physik, Universität Bonn, Wegelerstr. 8, D-53115 Bonn, Germany*

## SI. LOCAL ADDRESSING OF INDIVIDUAL ATOMS

The microwave addressing resolution of 20 lattice sites given in the main text limits the maximum number of atoms that we can sort in a low-entropy state. Our imaging system's field of view spans over 160 lattice sites, which corresponds to 8 atoms separated by 20 sites. However, the situation of 8 atoms equally separated is extremely improbable since atoms are initially distributed in random positions. Thus, with the experimental apparatus presently at hand we are limited to between 4 and 6 atoms.

With the same experimental apparatus, we have demonstrated in the past much higher addressing resolutions, by working with magnetic field gradients about a factor 20 higher [28]. The technical challenge using high magnetic field gradients resides in the long time (more than 100 ms) required to ramp up or down the magnetic field, during which off-resonant scattering of lattice photons can occur ($T_1 \approx 100\,\mathrm{ms}$). This is not a problem for atoms sorted in distinct lattice sites, since they can be reinitialized into the motional ground state by sideband cooling. However, it poses a limitation for sorting two or more ground-state-cooled atoms into the same lattice site, since the subsequent application of sideband cooling would lead to highly detrimental losses by light-assisted collisions instead of reinitializing atoms into the ground state. Hence, for our atom-sorting demonstration, we opted for a rather weak magnetic field gradient, which enables in the future the study of intriguing many-body effects.

Moreover, switching from magnetic field gradients to tightly focused laser beams employing a high-NA objective lens [44] should allow us to achieve local addressing with single-lattice-site resolution.

| | Conservative | State of the art |
|---|---|---|
| Image acquisition time | 60 ms | 30 ms |
| Addressing efficiency | 80 % | 95 % |
| Addressing crosstalk | 10 % | 5 % |
| Initial filling probability | 40 % | 60 % |
| Storage time | 60 s | 360 s |
| Duration of optical pumping | 10 ms | 10 ms |
| Duration of lattice shift | 1 ms | 1 ms |
| Addressing duration | 150 µs | 30 µs |

TABLE. S1. Monte Carlo simulation parameters of PSOLAS for a conservative and a state-of-the-art scenario, as described in Sec. SII.

* alberti@iap.uni-bonn.de; †Both authors contributed equally to this work.

## SII. MONTE CARLO SIMULATIONS OF PSOLAS

We carried out Monte Carlo simulations of the PS-optical-lattice atom-sorting (PSOLAS) algorithm using the parameters reported in Tab. S1 for two different scenarios based on either conservative or state-of-the-art conditions. As mentioned in the main text, we have chosen the conditions of both scenarios based on individual results obtained either in our or other laboratories.

We are currently setting up a two-dimensional (2D) polarization-synthesized (PS) optical lattice experimental apparatus, which is designed to reach the experimental conditions described in the state-of-the-art scenario [45]. A key component of our new experimental apparatus is a custom-built objective lens with high numerical aperture NA=0.92 [44]. The objective lens achieves a diffraction limited resolution of 460 nm, compared to the lattice constant of 612 nm, and increases the photon collection efficiency by a factor 30 compared to that obtained with the apparatus described in the main text. Consequently, we expect a significant improvement in the localization precision, allowing us to determine the lattice position of individual atoms in few tens of milliseconds. Furthermore, the high-NA objective lens should enable us to address individual atoms with high efficiency using tightly focused laser beams, which induces a differential light shift for the addressed atoms [50]. It was recently demonstrated that the efficiency of this technique can exceed 99 % [8]. Thus, we assumed in our Monte Carlo simulations an addressing efficiency of 80 % and 95 % for the two scenarios. We additionally accounted for an addressing crosstalk of 5 % or 10 %, which leads to unwanted spin flips of neighboring atoms. Moreover, the region of $100\times100$ sites considered in the Monte Carlo simulations corresponds to the field of view of our high-NA objective lens.

The initial filling probability of the lattice is determined by the density of atoms that are initially captured in the magneto-optical trap and by the efficiency of the so-called parity projection caused by light-assisted collisions. In our current implementation we found initial filling probabilities to vary between 40 % and 65 %. Notably, Fung *et al.* [20] show that initial filling probabilities exceeding 80 % can be realized using an additional blue-detuned laser beam while loading atoms from the magneto-optical trap into the optical lattice.

With the experimental apparatus described in the main text, we achieve storage times in the range of 360 s due to the ultra-high vacuum conditions realized in the "science" cell, where the partial vacuum pressure of Cs atoms is very low. With the new 2D experimental apparatus, we expect to achieve storage times of the order of one minute.

The chosen duration of optical pumping (10 ms) and that of a lattice shift operation (1 ms) match the settings of the experiments reported in the main text. For serial

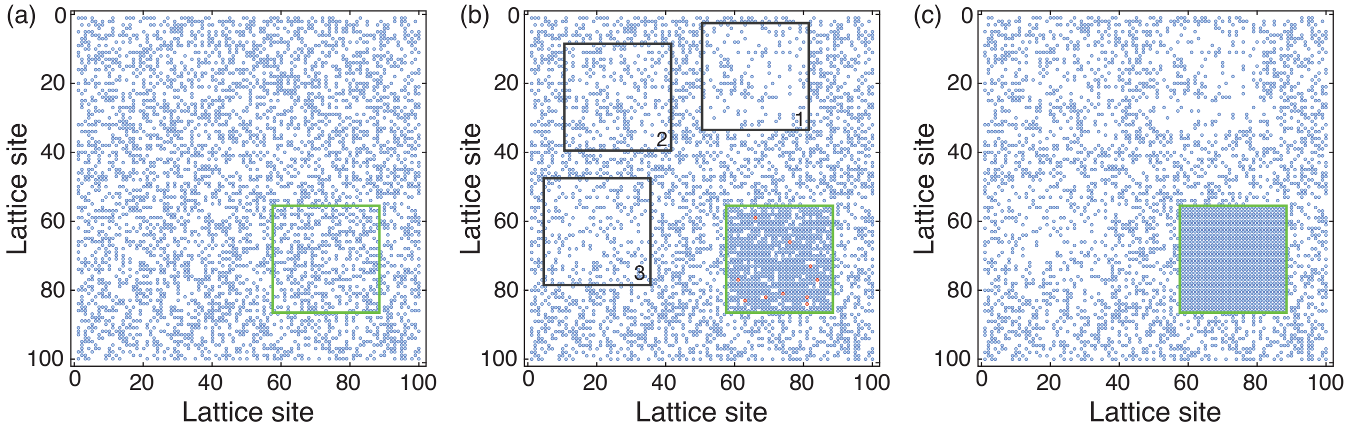


FIG. S1. Conceptual illustration of PSOLAS using the conservative parameters given in Tab. S1. The goal is to create unity filling in a square target pattern of 31 × 31 lattice sites (green square region). (a) Initial distribution of atoms in a 2D optical lattice with 40 % initial filling probability. (b) Atom distribution after 3 PSOLAS iterations. The black squares represent the regions where the atom patterns best matched the remaining holes in the target region. The red pixels indicate lattice sites with double occupancy, which are caused from addressing crosstalk at the third iteration of PSOLAS. In our Monte Carlo simulations, we assumed perfect parity projection; hence these lattice sites will result in holes at the next iteration of PSOLAS. (c) Final atom distribution with unity filling of 961 lattices sites (31 × 31) obtained after 12 PSOLAS iterations.

addressing, the addressing duration depends on how fast one can steer the laser beam generating the local differential light shift and the duration of the subsequently applied microwave pulse itself. Previous demonstrations of the addressing scheme achieved local differential light shifts of ≈ 60 kHz [50]. In this case, microwave pulses with a duration of 30 µs have the required frequency resolution to ensure low addressing crosstalk. As a conservative assumption, we take the current microwave pulse duration of 150 µs, which correspond to smaller AC stark-shifts. In both scenarios, the beam steering duration can be neglected due to the high bandwidth of acousto-optic modulators (steering time < 1 µs). Furthermore, we note that spatial light modulators [48, 49] (e.g., liquid crystal on silicon operated in amplitude modulation mode, with refresh rates of $\gtrsim$ 10 Hz) could also enable parallel addressing of hundreds of atoms by imaging the square grid of pixels onto the square two-dimensional optical lattice.

For the complexity estimate of PSOLAS, we neglected the computational time required to process, e.g., atom positions, which can be efficiently performed by a CPU or in parallel by a dedicated FPGA chip. This computational time is much shorter than the other time scales.

## SIII. ILLUSTRATION OF PSOLAS

In Fig. S1, we provide a graphical illustration of the working principle of PSOLAS algorithm under the conservative conditions (see Tab. S1) to accompany the description given in the main text. For the chosen example, we use PSOLAS to create unity filling in a square target pattern of 31 × 31 lattice sites, repositioning atoms taken from within a region of 100 × 100 lattice sites. The three images in the figure are Monte Carlo-simulated atom distributions at the initial time, after three iterations of the algorithm, and at the completion of the algorithm. The initial distribution, see Fig. S1(a), is a random distribution of atoms with an initial filling probability of 40 %. PSOLAS chooses the initially densest region of 31 × 31 lattice sites as the target region, which is indicated by a green rectangle in the figure. The atom distribution after three iterations, see Fig. S1(b), shows a highly increased density in the target region, whereas a visible depletion in the other square regions indicated by numbers 1, 2, 3, identified by PSOLAS as those regions with atom patterns best matching the distribution of the remaining holes of the target region. In Fig. S1(c), we show the final distribution with perfect unity filling in the target region after 12 iterations of PSOLAS algorithm.

## BIBLIOGRAPHY


[8] Y. Wang, A. Kumar, T. Y. Wu, and D. S. Weiss, "Single-qubit gates based on targeted phase shifts in a 3D neutral atom array," Science **352**, 1562 (2016).

[20] Y. Fung, P. Sompet, and M. Andersen, "Single Atoms Preparation Using Light-Assisted Collisions," Technologies **4**, 4 (2016).

[28] M. Karski, L. Förster, J. Choi, A. Steffen, N. Belmechri, W. Alt, D. Meschede, and A. Widera, "Imprinting Patterns of Neutral Atoms in an Optical Lattice using Magnetic Resonance Techniques," New J. Phys. **12**, 065027 (2010).

[44] C. Robens, S. Brakhane, W. Alt, F. Kleißler, D. Meschede, G. Moon, G. Ramola, and A. Alberti, "A high numerical aperture (NA = 0.92) objective lens for imaging and addressing of cold atoms," arXiv (2016), arXiv:1611.02159 [physics.ins-det].

[45] T. Groh, S. Brakhane, W. Alt, D. Meschede, J. K. Asbóth, and A. Alberti, "Robustness of topologically protected edge states in quantum walk experiments with neutral atoms," Phys. Rev. A 94, 013620 (2016).

[48] G. Gauthier, I. Lenton, N. M. Parry, M. Baker, M. J. Davis, H. Rubinsztein-Dunlop, and T. W. Neely, "Direct imaging of a digital-micromirror device for configurable microscopic optical potentials," Optica **3**, 1136 (2016).

[49] F. Nogrette, H. Labuhn, S. Ravets, D. Barredo, L. Béguin, A. Vernier, T. Lahaye, and A. Browaeys, "Single-Atom Trapping in Holographic 2D Arrays of Microtraps with Arbitrary Geometries," Phys. Rev. X 4, 021034 (2014).

[50] C. Weitenberg, M. Endres, J. F. Sherson, M. Cheneau, P. Schauß, T. Fukuhara, I. Bloch, and S. Kuhr, "Single-spin addressing in an atomic Mott insulator," Nature 471, 319 (2011).
